# Supplementary material for: Query Resolution for Conversational Search with Limited Supervision
Source: arXiv:2005.11723 source file (2020-05-24)
Supplement: Supplementary file 1 [file appendix.tex]

%!TEX root = ./main.tex
\appendix

\section{Conversation examples}
Table~\ref{tab:quac_paragraph2} shows another example dialogue.
\begin{table}[t]
	\centering
	
	\caption{Excerpt from an example dialogue taken from the QuAC training data. 
	%The paragraph originates from the section ``History'' of the Wikipedia article on ``Saosin''. 
	Terms in boldface are the overlapping terms between turns \#1-5 and the answer to the current turn query (\#6). Those overlapping terms are relevant to the current turn query.
	%We denote the answer spans of each query turn in the paragraph with a superscript.
	}
	\begin{tabular}{p{1.5cm} p{5cm}}
		\toprule
%        \textbf{Turn} & \multicolumn{1}{c}{\textbf{Query} }
        \textbf{Turn} & \textbf{Query}
        \\\midrule
        	%   What singles came from that album?
		1 & Was death of a Ladies man an album?? \\
		2 & Who performed if he cowrote and produced? \\
		3 & What this album \textbf{successful}? \\
		4 &  What can you tell me about \textbf{End of the Century} album? \\
		5 & What \textbf{singles} came from that album?
	\\
		6 (current) & Was this album a success? \\
%		\ldots & \ldots \\
		\midrule
		\multicolumn{2}{p{0.95\linewidth}}{\textit{
		Answer to turn \#6}: \ldots the much-publicized Ramones album \textbf{End of the Century} in 1979. As with his work with Leonard Cohen, End of the Century received criticism from Ramones fans who were angered over its radio-friendly sound. However, it contains some of the best known and most \textbf{successful} Ramones \textbf{singles}, such as Rock 'n' Roll High School, Do You Remember Rock 'n' Roll Radio? \ldots
		}\\
        \bottomrule
	\end{tabular}
	\label{tab:quac_paragraph2}
\end{table}
